# Supplementary material for: Learning curves of generic features maps for realistic datasets with a teacher-student model
Source: arXiv:2102.08127 source file (2021-12-14)
Supplement: Supplementary file 1 [file scaling_ridge.tex]

In this appendix we derive the scaling results from \cite{spigler2019asymptotic, bordelon2020} for the decay of the generalisation error in kernel ridge regression directly from our framework.

As discussed in Appendix \ref{sec:app:connection}, kernel ridge regression can be written as ridge regression in feature space, see eqs.~\eqref{eq:app:kernel}. Here, we are interested in understanding how the generalisation error depends on the decay of the teacher weights and of the student covariance $\Omega$, in the case considered in \cite{bordelon2020, spigler2019asymptotic} where the student dimension is infinity $\sdim=\infty$. 

We remind that in the kernel ridge regression case, the saddle point equations read:
\begin{align}
\label{eq:app:SP_kernel}
    \begin{cases}
        \hat{V} = \hat{m} = \frac{\alpha}{1+V}\\
        \hat{q} = \alpha\frac{\rho+q-2m}{(1+V)^2}\\
    \end{cases}, && 
    \begin{cases}
		V =  \frac{1}{\sdim}\sum\limits_{i=1}^{d}\frac{\omega_{i}}{\lambda + \hat{V}\omega_{i}}\\
		q = \frac{1}{\sdim}\sum\limits_{i=1}^{d}\frac{\hat{q}\omega_{i}^2+\tilde{\theta}_{i}\omega_{i} \hat{m}^2}{(\lambda+\hat{V}\omega_{i})^2}\\
		m=\frac{\hat{m}}{\sdim}\sum\limits_{i=1}^{d}\frac{\omega_{i}\tilde{\theta}_{i}}{\lambda+\hat{V}\omega_{i}}
	\end{cases},
\end{align}
\noindent where we have defined $\tilde{\theta}_{i} = \theta_{0i}^2\omega_{i}$ for convenience, with $\omega_i$ being the $i^{\rm{th}}$ eigenvalue of the student covariance $\Omega$. In subsection \ref{subsection:app:selfconsistent}, we derive a pair of coupled self-consistent equations determining the generalization error $\epsilon_g$, which we simplify in the $\sdim\rightarrow\infty$ limit in subsection\ref{subsection:app:dinf} and extract therefrom the asymptotic behaviour for $\epsilon_g$ in subsection \ref{subsection:app:nbig} as $n\gg1$.

\subsection{Self-consistent equations for the generalization error}
\label{subsection:app:selfconsistent}
Define $z = \alpha \frac{\lambda}{\hat{V}}$. Note that we can find a closed equation for $z$ by combining the equations for $(\hat{V},V)$:
\begin{align}
z \equiv \alpha \frac{\lambda}{\hat{V}} = \alpha \frac{\lambda}{\alpha} (1+V) = \lambda+\frac{1}{ d}\sum\limits_{i=1}^{p}\frac{\lambda\omega_{i}}{\lambda+\hat{V}\omega_{i}}.
\end{align}
Therefore:
\begin{equation}
\label{eq:app:z}
z = \lambda+\frac{z}{n}\sum\limits_{i=1}^{d}\frac{\omega_{i}}{\frac{z}{\alpha }+\omega_{i}}.
\end{equation}

The test error is given by $\epsilon_{g} = \rho+q-2m$. Using the saddle-point equations \eqref{eq:app:SP_kernel}, we can write:
\begin{align}
\epsilon_{g} &\underset{(a)}{=} \frac{1}{d}\sum\limits_{i=1}^{d}	\left[\tilde{\theta}_{i}+\frac{\hat{q}\omega_{i}^2+\tilde{\theta}_{i}\omega_{i}\hat{m}^{2}}{(\lambda+\hat{V}\omega_{i})^2} - \frac{2\hat{m}\tilde{\theta}_{i}\omega_{i}}{\lambda+\hat{V}\omega_{i}}\right]\notag\\
&\underset{(b)}{=} \frac{1}{d}\sum\limits_{i=1}^{d}\frac{\left(\lambda+\hat{V}\omega_{i}\right)^2+\alpha^{-1}\omega_{i}^2\hat{V}^{2}\epsilon_{g}+\hat{V}^{2}\tilde{\theta}_{i}\omega_{i}-2\tilde{\theta}_{i}\hat{V}\omega_{i}\left(\lambda+\hat{V}\omega_{i}\right)}{(\lambda+\hat{V}\omega_{i})^2}\noindent\\
&= \frac{1}{d}\sum\limits_{i=1}^{d}\frac{\alpha^{-1}\omega_{i}^2\hat{V}^{2}\epsilon_{g}+\lambda^2\tilde{\theta}_{i}}{(\lambda+\hat{V}\omega_{i})^2},
\end{align}
\noindent where in $(a)$ we simply used the equations for $q,m$ and the definition of $\rho$ and in $(b)$ we used $\hat{m}=\hat{V}$ and $\hat{q}=\alpha^{-1}\hat{V}^2\epsilon_{g}$. Note that the right-hand side now only depends on the overlap $\hat{V}$. Solving for $\epsilon_{g}$ and writing everything as a function of $z = \alpha\lambda/\hat{V}$:
\begin{equation}
\label{eq:app:kernelridge_gen_error}
\epsilon_{g} = \frac{\frac{z^2 d}{n ^2 }\sum\limits_{i=1}^{d}\frac{\tilde{\theta}_{i}}{\left(z\frac{d}{n}+\omega_{i}\right)^2}}{1-\frac{1}{n}\sum\limits_{i=1}^{d}\frac{\omega_{i}^2}{(z\frac{d}{n}+\omega_{i})^2}}.
\end{equation}

\noindent Equation \eqref{eq:app:kernelridge_gen_error} together with equation \eqref{eq:app:z} make for a pair of coupled equations whose solution allows to determine $\epsilon_g$. As written, solving for \eqref{eq:app:z} and \eqref{eq:app:kernelridge_gen_error} is not tractable. We show in subsection \ref{subsection:app:dinf} how the expressions \eqref{eq:app:z} and \eqref{eq:app:kernelridge_gen_error} simplify as the $\sdim\rightarrow\infty$ limit is taken. In subsection \ref{subsection:app:nbig}, we further show how in the $n\gg 1$ regime the asymptotic behaviour for the generalization error \eqref{eq:app:kernelridge_gen_error} can be extracted.

\subsection{Limit of infinite student dimension}
\label{subsection:app:dinf}
Now assume the following power law decay for the covariance $\Omega$ and the teacher $\vec{\theta}_{0}$:
\begin{align}
\label{eq:app:decayansatz}
\omega_i=i^{-b}\sdim, && \tilde{\theta}_i=i^{-a}\sdim,
\end{align}
i.e. the eigenvalues of $\Omega$ possess a power-law decay with exponent $b$, while the components of the teacher $\theta_{0i}$ decay with exponent $\frac{a-b}{2}$. Note that ansatz \eqref{eq:app:decayansatz} slightly differs from the one assumed in \cite{bordelon2020,spigler2019asymptotic} by a factor $\sdim$, resulting from differing normalization conventions in the loss considered. Since labels $y^\mu=\frac{1}{\sqrt{d}}\theta_0\cdot x^\mu$ are defined with a normalization $\sqrt{d}$ in the present work, the factor $\sdim$ is necessary in \eqref{eq:app:decayansatz} to keep labels of $\mathcal{O}(1)$.
\noindent Then equation \eqref{eq:app:kernelridge_gen_error} can be simplified to
\begin{equation}
\epsilon_{g} = \frac{\frac{z^2 }{n ^2 }\sum\limits_{i=1}^{d}\frac{i^{-a}}{\left(z\frac{1}{n}+i^{-b}\right)^2}}{1-\frac{1}{n}\sum\limits_{i=1}^{d}\frac{i^{-2b}}{(z\frac{1}{n}+i^{-b})^2}},
\end{equation}
which has a meaningful limit as $d\rightarrow \infty$ (with $n$, $\lambda$ kept fixed):
\begin{equation}
\epsilon_{g} = \frac{\sum\limits_{i=1}^{\infty}\frac{i^{-a}}{\left(1+nz^{-1}i^{-b}\right)^2}}{1-\frac{n}{z^2}\sum\limits_{i=1}^{\infty}\frac{i^{-2b}}{1+nz^{-1}i^{-b})^2}}.
\end{equation}
In the same limit, the equation defining $z$ \eqref{eq:app:z} is amenable to being rewritten:
\begin{equation}
\label{eq:app:z2}
  z=\lambda +\frac{z}{\samples }\sum\limits_{i=1}^\infty \frac{1}{1+\frac{z}{\samples }i^b} .
\end{equation}

\subsection{Infinite sample limit and the scaling of the generalisation error}
\label{subsection:app:nbig}
Consider now the limit $n\gg 1$ with $\lambda$ kept fixed. We can use a Riemann approximation to rewrite \eqref{eq:app:z2} in integral form, for $n\gg1$: 
\begin{align}
\label{eq:app:z3}
    z&\approx \lambda+\left(\frac{z}{\samples }\right)^{1-\frac{1}{b}}\int_{\left(\frac{z}{\samples }\right)^{1/b}}^\infty \frac{\dd x}{1+x^b}.
\end{align}
Note that the scalings of $z$ with respect to $\samples$ differ according to the regularisation $\lambda$, depending on which of the two terms on the right hand side of equation \eqref{eq:app:z3} dominates. If the first $\lambda$ term dominates, then \eqref{eq:app:z3} simplifies to $z\approx\lambda$. For this to be self-consistent, we must have $(z/n)^{1-\frac{1}{b}}\approx(\lambda/n)^{1-\frac{1}{b}}\ll\lambda$, i.e. $n\gg \lambda^{-\frac{1}{b-1}}$. In the converse case where the second term in \eqref{eq:app:z3} dominates, $z\sim \samples ^{1-b}$. For this to consistently hold, one needs $(z/n)^{1-\frac{1}{b}}\approx n^{1-b}\gg\lambda$, i.e. $n\ll \lambda^{-\frac{1}{b-1}}$. Therefore there exist in total two regimes:
\begin{itemize}
    \item in the $n\ll \lambda^{-\frac{1}{b-1}}$ regime, $z\sim \samples ^{1-b}$,
    \item in the $n\gg \lambda^{-\frac{1}{b-1}}$ regime, $z\approx \lambda$.
\end{itemize}
In the first regime, the numerator of $\epsilon_g$ reads possesses different scalings according to exponents $a,b$. if $2b-a>-1$, \begin{align}
   \sum\limits_{i=1}^{\infty}
    \frac{i^{-a}}{(1+\samples z^{-1}i^{-b})^2}&\sim
    \samples ^{1-a}\sum\limits_{i=1}^{\infty}
    \frac{\left(\frac{i}{\samples }\right)^{-a}}{(1+\left(\frac{i}{n}\right)^{-b})^2}\frac{1}{\samples }
    \sim \samples ^{1-a}\int\limits_0^\infty \frac{x^{2b-a}}{(1+x^b)^2}=\mathcal{O}(\samples ^{1-a}).
\end{align}
If $2b-a<-1$, it is no longer possible to write the Riemann sum as an integral, and 
\begin{align}
   \sum\limits_{i=1}^\infty
    \frac{i^{-a}}{(1+\samples z^{-1}i^{-b})^2}&=
    \sum\limits_{i=1}^\samples 
    \frac{i^{-a}}{(1+\samples ^bi^{-b})^2}
    +
    \samples ^{1-a}\sum\limits_{i=\samples }^\infty
    \frac{\left(\frac{i}{\samples }\right)^{-a}}{(1+\left(\frac{i}{n}\right)^{-b})^2}\frac{1}{\samples }=\mathcal{O}(\samples ^{-2b}).
\end{align}
It is possible to similarly decompose the sum in the denominator to find
\begin{equation}
    \frac{\samples }{z^2}\sum\limits_{i=1}^{\infty}
    \frac{i^{-2b}}{(1+\samples z^{-1}i^{-b})^2}=\mathcal{O}(1).
\end{equation}
From this, it follows that:
\begin{equation}
\label{eq:app:scaling1}
    \epsilon_g=\mathcal{O}\left(\samples ^{-\rm{min}(a-1,2b)}\right)
\end{equation}
By the same token, in the second $n\gg \lambda^{-\frac{1}{b-1}}$ regime,provided $2b-a>-1$, one can write the numerator as a Riemann sum:

\begin{align}
   \sum\limits_{i=1}^{\infty}
    \frac{i^{-a}}{(1+\samples z^{-1}i^{-b})^2}&\sim
    \left(\frac{\lambda}{\samples }\right)^{\frac{a-1}{b}}
    \sum\limits_{i=1}^{\infty}\frac{\left(i\left(\frac{\lambda}{\samples }\right)^{\frac{1}{b}}\right)^{2b-a}}{\left(\left(i\left(\frac{\lambda}{\samples }\right)^{\frac{1}{b}}\right)^b+1\right)^2}\left(\frac{\lambda}{\samples }\right)^{\frac{1}{b}}\sim \left(\frac{\lambda}{\samples }\right)^{\frac{a-1}{b}}\int\limits_0^\infty \frac{x^{2b-a}}{(1+x^b)^2}=\mathcal{O}(\samples ^{\frac{1-a}{b}}).
\end{align}
In the $2b-a<-1$ case, 
\begin{align}
   \sum\limits_{i=1}^\infty
    \frac{i^{-a}}{(1+\samples z^{-1}i^{-b})^2}&=
    \sum\limits_{i=1}^{\samples ^\frac{1}{b}}
    \frac{i^{-a}}{(1+\frac{\samples }{\lambda}i^{-b})^2}
    +
    \left(\frac{\lambda}{\samples }\right)^{\frac{a-1}{b}}
    \sum\limits_{i=\samples ^\frac{1}{b}}^\infty\frac{\left(i\left(\frac{\lambda}{\samples }\right)^{\frac{1}{b}}\right)^{2b-a}}{\left(\left(i\left(\frac{\lambda}{\samples }\right)^{\frac{1}{b}}\right)^b+1\right)^2}\left(\frac{\lambda}{\samples }\right)^{\frac{1}{b}}.
\end{align}
Upper and lower bounds can be straightfowardly found for the first sum and the following equivalence established
\begin{equation}
    \sum\limits_{i=1}^{\samples ^\frac{1}{b}}
    \frac{i^{-a}}{(1+\frac{\samples }{\lambda}i^{-b})^2}
    \sim \samples ^{-2}\sum\limits_{i=1}^{\samples ^\frac{1}{b}}i^{2b-a}=\mathcal{O}(\samples ^{-2}),
\end{equation}
while the second sum is a Riemann sum of order $\mathcal{O}(\samples ^\frac{1-a}{b})=o(\samples ^{-2})$. Finally, the scaling of the sum in the denominator is found along similar lines to be 
\begin{equation}
    \frac{\samples }{z^2}\sum\limits_{i=1}^{\infty}
    \frac{i^{-2b}}{(1+\samples z^{-1}i^{-b})^2}=\mathcal{O}(\samples ^\frac{1-b}{b})=o(1).
\end{equation}
Putting everything together, 
\begin{equation}
\label{eq:app:scaling2}
    \epsilon_g=\mathcal{O}\left(\samples ^{-\frac{\rm{min}(a-1,2b)}{b}}\right).
\end{equation}

The scaling exponents \eqref{eq:app:scaling1} and \eqref{eq:app:scaling2} are in agreement with those derived through other means in \cite{bordelon2020}. \eqref{eq:app:scaling1} recovers the exponents derived using Fourier analysis in \cite{spigler2019asymptotic}, with $a=\frac{\alpha_T}{d},b=\frac{\alpha_S}{d}$ in their notations.
